# Supplementary material for: Statistical Inference for Complete and Incomplete Mobility Trajectories under the Flight-Pause Model
Source: arXiv:2210.07870 ancillary file (2023-06-30)
Supplement: Supplementary file 1 [file supplement.pdf]

# Supplementary material for ”Statistical Inference for Complete and Incomplete Mobility Trajectories under the Flight-Pause Model”

Marcin Jurek, Catherine Calder and Corwin Zigler

June 30, 2023

## S1 Sample trajectories and imputations used in numerical simulations

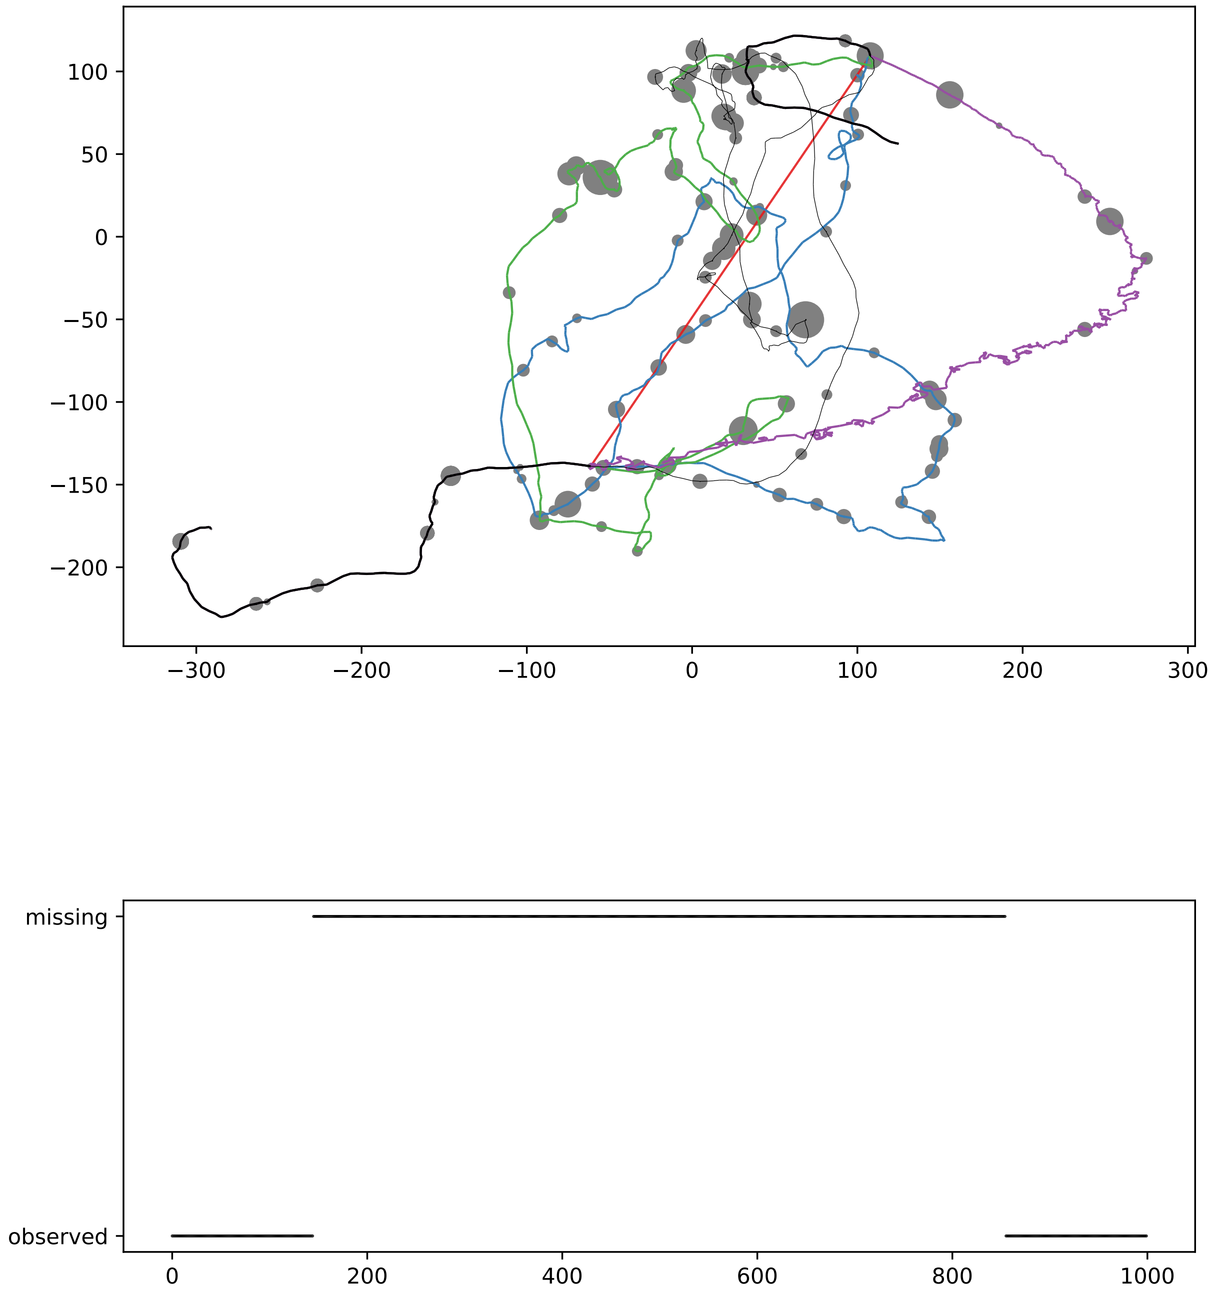


Figure S1: A sample trajectory and imputation with only unscheduled missingness (pattern shown in lower panel)

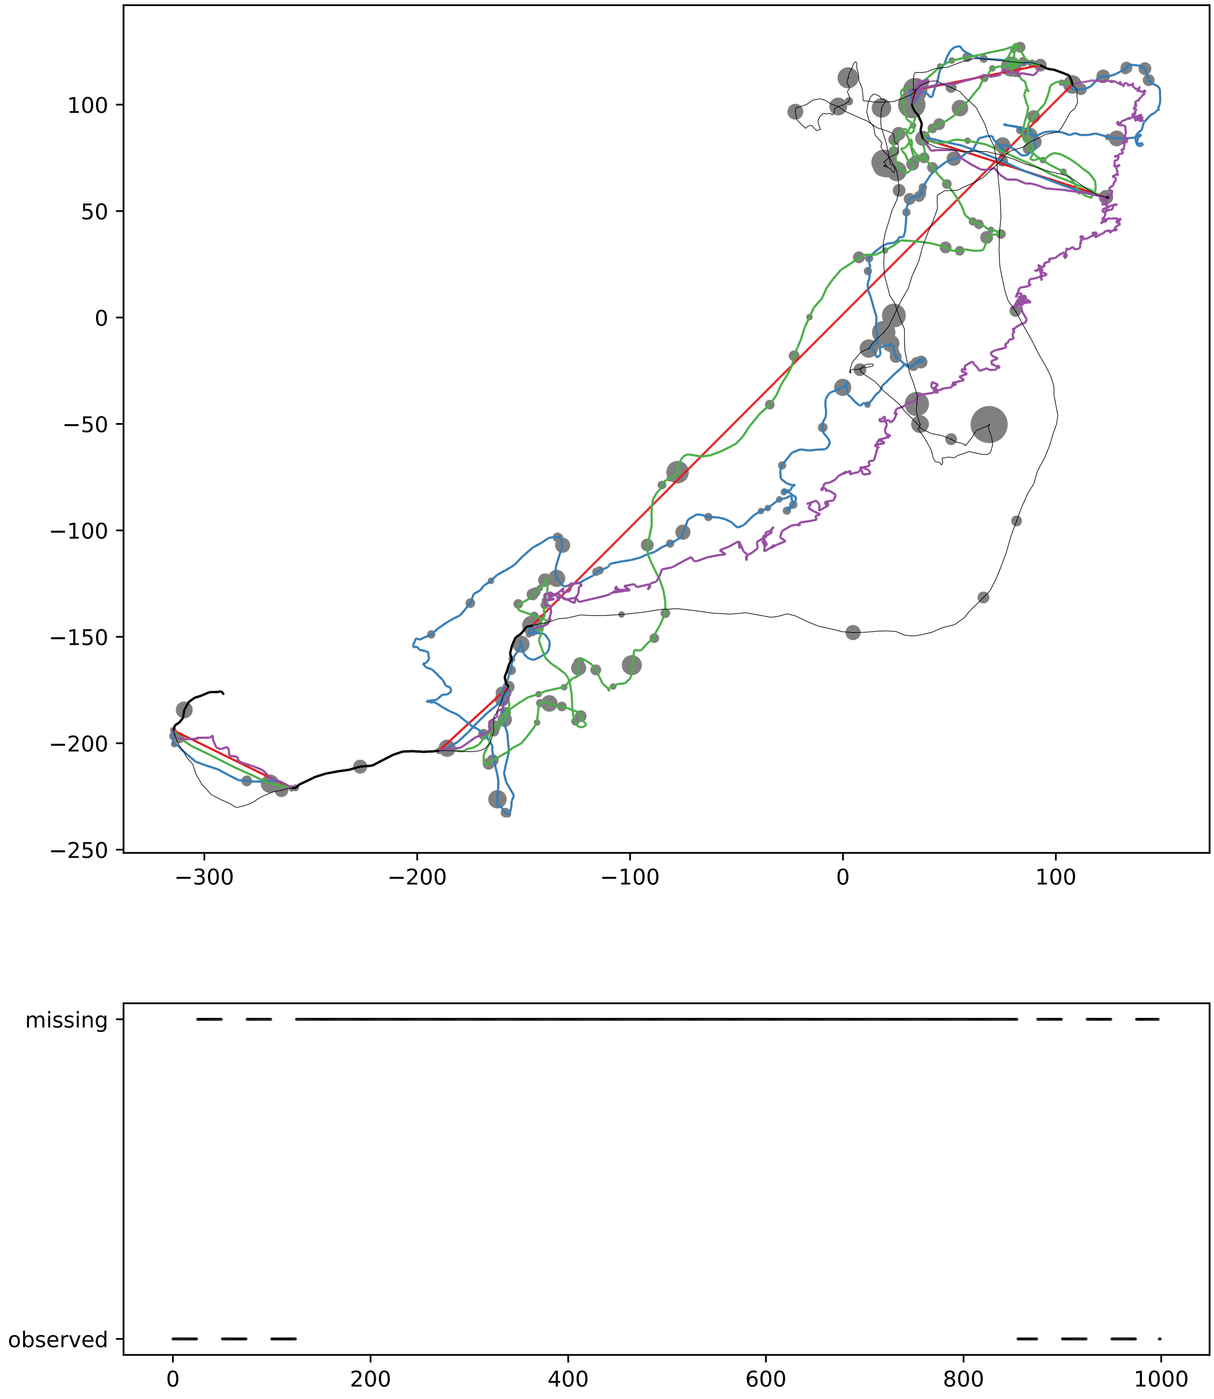


Figure S2: A sample trajectory and imputation with unscheduled missingness and short ”on” period (pattern shown in lower panel)

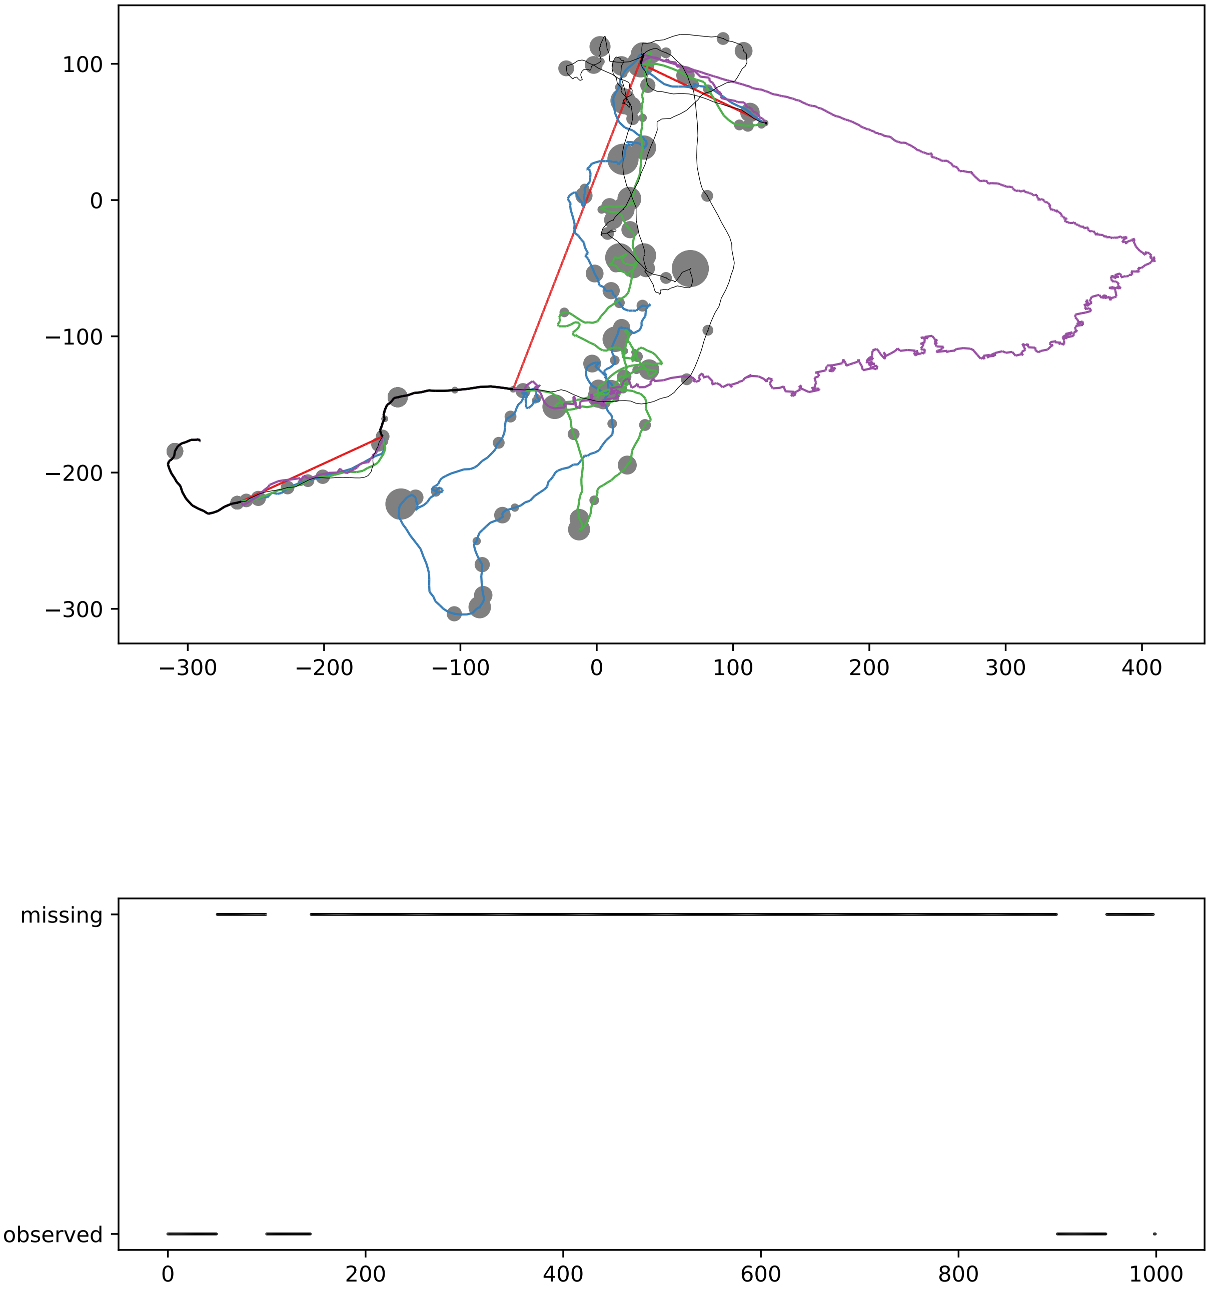


Figure S3: A sample trajectory and imputation with unscheduled missingness and long ”on” period (pattern shown in lower panel)

# S2 Other Results

A further improvement in sampling the unobserved blocks $U_j$ in Section 5 might be obtained if we use the following proposition to sample the increment types. We leave this as a direction for further research.

**Proposition 1.** *Let $\mathcal{F}_j = \mathcal{F} \cap U_j$ and $\mathcal{P}_j = \mathcal{P} \cap U_j$ The joint density of $|\mathcal{F}_|$ and $|\mathcal{P}_j|$, respectively, the number of flights and the number of pauses within a block $U_j$, is proportional to*

$$\binom{|\mathcal{F}_j|+2}{|\mathcal{F}_j|-|\mathcal{P}_j|+1}\binom{N_j-|\mathcal{F}_j|-3}{|P_j|+1} C\alpha_1^{|\mathcal{F}_j|-|\mathcal{P}_j|+1}\alpha_2^{|\mathcal{F}_j|+2},$$

*where* $C = \frac{(1-\theta_2)^{N_j+1}}{\theta_1(\theta_1+\theta_2)}$, $\alpha_1 = \frac{1-\theta_1}{\theta_1}\frac{1-\theta_2}{\theta_2}$ *and* $\alpha_2 = \frac{\theta_1^2\theta_2}{1-\theta_2}$.

The proof of Proposition 1 requires the following

**Fact 1.** *In each observed block $O_j$ both the first and last increments are flights.*

*Proof of Fact 1:* By Proposition 1 observing a pause requires information about its preceding increment. Thus the first increment in an observed block cannot be a pause so it has to be a flight. Moreover, in order to observe a pause we also need to know the trajectory of the flight that follows it as well as the first location in the increment following that flight. Thus a pause can never be the last observed increment in a given block. □

*Proof of Proposition 1.* Let $q_t = \mathbb{1}(t \in \mathcal{D}(\mathcal{F}))$ (notice this is different than before but it leads to cleaner algebra). We can then consider the type and duration of increments in $\boldsymbol{M}_{I_j+N_j-1} \cup U_j \cup \boldsymbol{M}_{I_{j+1}}$ to be represented by a two-state Markov chain

$$\{q_t\}_{L^T_{I_j+N_j-1}}^{L^T_{I_{j+1}}}.$$

Let us define $p_{11} = \sum_{L^T_{I_j+N_j}}^{L^T_{I_{j+1}}} q_t q_{t-1}$ and $p_1 = \sum_{L^T_{I_j+N_j-1}}^{L^T_{I_{j+1}}} q_t$. Intuitively, $p_{11}$ is the number of transitions from state 1 back to state 1, while $p_1$ is the total time spent in state 1. Define also $\bar{p} = q_{L^T_{I_{j+1}}} + q_{L^T_{I_j+N_j-1}}$. Klotz (1973) derive an expression for the joint distribution of $p_{11}, p_1$ and $\bar{p}$ as

$$q(p_{11},p_1,\bar{p}) = \binom{2}{\bar{p}}\binom{p_1}{p_{11}}\binom{N_j-p_1-1}{p_1-p_{11}-\bar{p}}(1-\theta_2)^{N_j-1}\frac{\theta_1}{\theta_1+\theta_2}\left(\frac{1-\theta_1}{\theta_1}\frac{1-\theta_2}{\theta_2}\right)^{p_{11}}\left(\frac{\theta_1^2\theta_2}{1-\theta_2}\right)^{p_1}\left(\frac{1-\theta_2}{\theta_1}\right)^{\bar{p}}.$$

Notice that in our case $\bar{p} = 1$ because as shown in Fact 1 the first last increment in $I_j$ and the first increment in $I_{j+1}$ are flights. Furthermore, observe that $p_1 = |F_j| + 2$, while $p_{11} = |F_j| - |P_j| + 1$. Thus, changing the variables we can write, that

$$q(p_{11},p_1|\bar{p}=2) = \binom{p_1}{p_{11}}\binom{N_j-p_1-1}{p_1-p_{11}-2}\frac{\theta_1}{\theta_1+\theta_2}\left(\frac{1-\theta_1}{\theta_1}\frac{1-\theta_2}{\theta_2}\right)^{p_{11}}\left(\frac{\theta_1^2\theta_2}{1-\theta_2}\right)^{p_1}\left(\frac{1-\theta_2}{\theta_1}\right)^2 =$$

$$\binom{|F_j|+2}{|F_j|-|P_j|+1}\binom{N_j-|F_j|-3}{|P_j|+1}(1-\theta_2)^{N_j-1}\left(\frac{1-\theta_1}{\theta_1}\frac{1-\theta_2}{\theta_2}\right)^{|F_j|-|P_j|+1}\left(\frac{\theta_1^2\theta_2}{1-\theta_2}\right)^{|F_j|+2}\left(\frac{1-\theta_2}{\theta_1}\right)^2.$$

□

# S3 Detailed simulation results

If for a given method $\nu$ and gap size $\alpha$ fractions $w_n^{\alpha,\nu,\zeta}$ or $v_n^{\alpha,\nu,\zeta}$ are the same for several trajectories $\tau(\Updownarrow_n)$, then the dot at the corresponding spot is larger in size. Note that for $\nu = LI$ (linear interpolation) each imputation is the same, which means that $w_n^{\alpha,\mathrm{LI},\zeta}, v_n^{\alpha,\mathrm{LI},\zeta} \in \{0,1\}$.

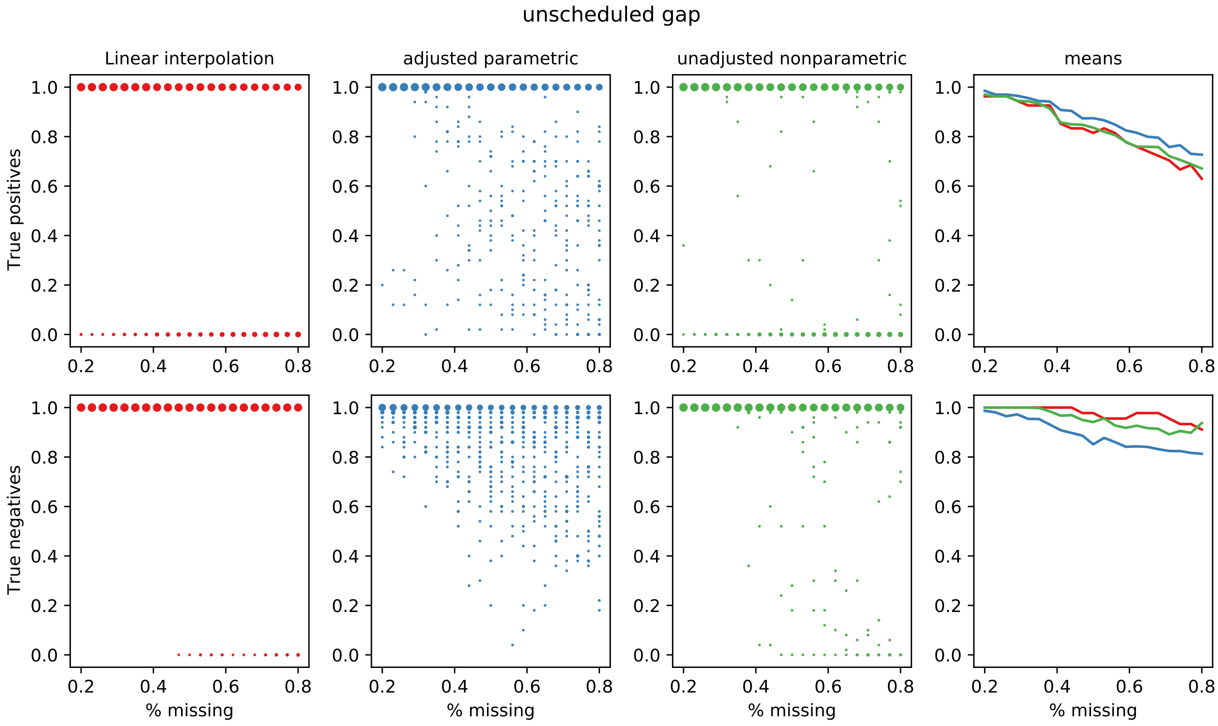


Figure S4: Probability of (not) passing through the hot-spot as a function of the percentage of the data which were missing.

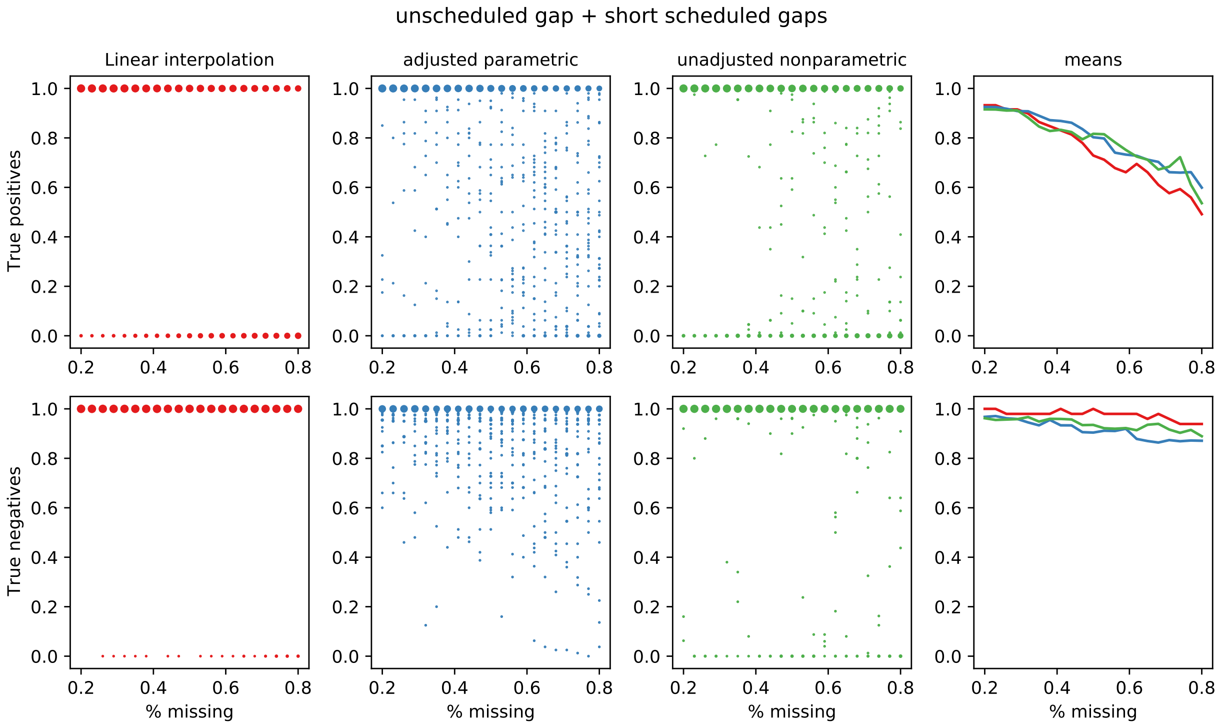


Figure S5: Probability of (not) passing through the hot-spot as a function of the length of the data which were missing outside of the schedule. The schedule prescribes that the data should be collected for $I_o = 25$ and then to not be collected for $I_u = 25$.

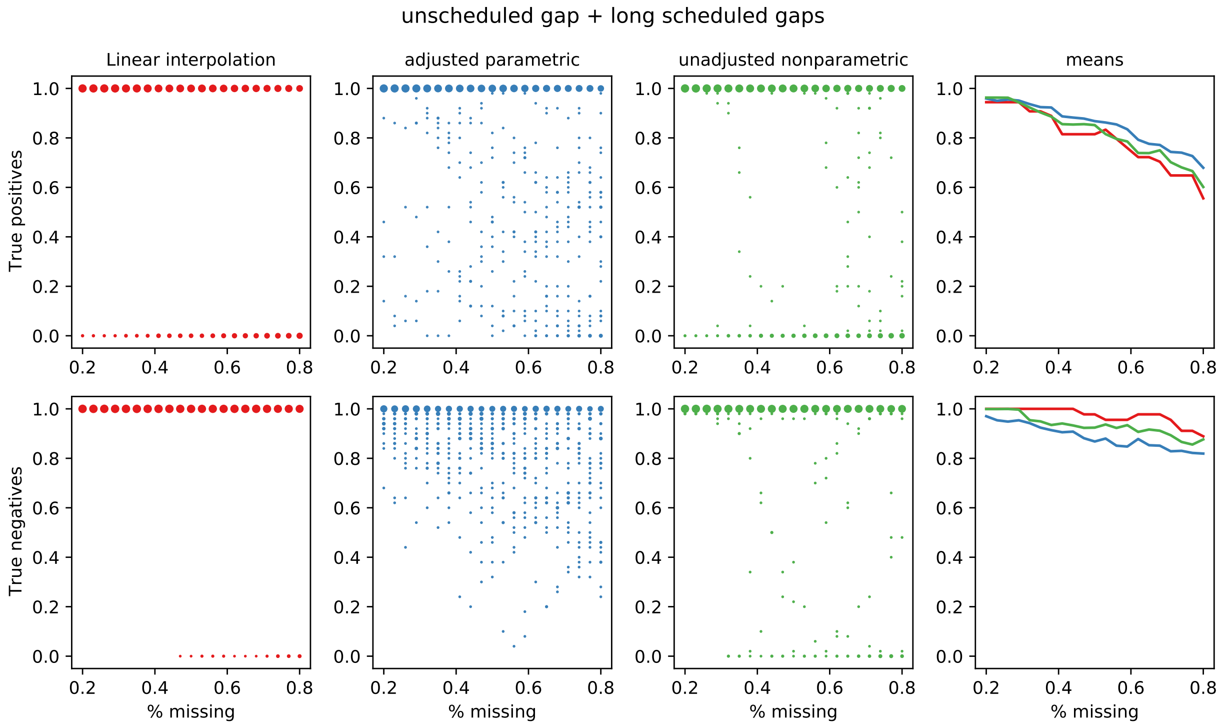


Figure S6: Probability of (not) passing through the hot-spot as a function of the length of the data which were missing outside of the schedule. The schedule prescribes that the data should be collected for $I_o = 50$ and then to not be collected for $I_u = 50$.

# References

Klotz, J. (1973). Statistical inference in bernoulli trials with dependence. *The Annals of statistics*, pages 373–379.
